# Supplementary material for: Phase transitions beyond criticality: extending Ising universal scaling functions to describe entire phases
Source: arXiv:2402.18531 ancillary file (2024-08-04)
Supplement: Supplementary file 1 [file sm.pdf]

# Supplemental Material for “Phase transitions beyond criticality: extending Ising universal scaling functions to describe entire phases”

David Hathcock[1] and James P. Sethna[2]

[1] IBM T. J. Watson Research Center, Yorktown Heights, NY 10598, USA

[2] Laboratory of Atomic and Solid State Physics, Cornell University, Ithaca, New York 14853, USA

## S1. 2D ISING MODEL

### A. Expanding Onsager's solution: Nonlinear renormalization group flows

Onsager's solution for the zero-field free energy [main text, Eq. (2)] can be expressed as $f(t) = a(t)\log t^2 + b(t)$ where $a$ and $b$ are analytic functions of $t = T - T_c$. In practice, $a$ and $b$ are determined by perturbatively expanding around the critical point, $T_c$. As described in the main text, these analytic coefficients are related to the nonlinear scaling temperature $\tilde{t}(t)$ and analytic background $f_a(t)$ in the normal form free energy $\tilde{f}(\tilde{t}) = f(t) - f_a(t) = -\frac{1}{2}\tilde{t}^2 \log \tilde{t}^2$ via [main text, Eq. (3)],

$$a(t) = -\frac{1}{2}\tilde{t}(t)^2, \quad b(t) = \frac{1}{2}\tilde{t}(t)^2 \log(\tilde{t}(t)^2/t^2) + f_a(t). \tag{S1}$$

From the normal form RG flows,

$$\frac{d\tilde{f}}{d\ell} = 2\tilde{f} - \tilde{t}^2 \qquad \frac{d\tilde{t}}{d\ell} = \tilde{t}, \tag{S2}$$

we can then deduce the RG flows for physical temperature and free energy

$$\begin{aligned} \frac{df}{d\ell} &= 2f + \left[\frac{df_a(t)}{dt}\tilde{t}(t)\left(\frac{d\tilde{t}(t)}{dt}\right)^{-1} - \tilde{t}(t)^2 - 2f_a(t)\right] = 2f + \left[4a(t) + \frac{2a(t)b'(t)}{a'(t)} - 2b(t) - \frac{4a(t)^2}{ta'(t)}\right] \\ \frac{dt}{d\ell} &= \tilde{t}(t)\left(\frac{d\tilde{t}(t)}{dt}\right)^{-1} = \frac{2a(t)}{a'(t)}. \end{aligned} \tag{S3}$$

Taking $a(t)$ and $b(t)$ from Onsager's solution and expanding the above expressions order by order, we obtain the renormalization flow equations given in Table S1. We have computed the flow equations for each of the coordinates considered in the main text $t = T - T_c$, $x = X - X_c$, $v = V - V_c$ and $\tau = (1/\sinh 2\beta - \sinh 2\beta)/2$, where $X = \exp(-2/T)$

TABLE S1. Zero-field renormalization group flows for the 2D Ising model obtained from Onsager's solution for the free energy via Eq. (S3). Flows are expressed in each of the temperature coordinates $t$, $x$, $v$, and $\tau$. Temperature flows can be obtained analytically; to simplify the coefficients in the $t$-flow we express them in terms of $T_c = 2/\log(2+\sqrt{2})$. Coefficients in the free energy flows are given to four digits, but can easily be evaluated to much higher precision. Note that the temperature flows in $v$ and $\tau$ have only odd terms because they obey the dual symmetry of the 2D Ising model.

| | |
|---|---|
| $\frac{df}{d\ell} = 2f - 0.09664 - 0.1138t - 0.01351t^2 + 0.01164t^3 + O(t^4)$ <br> $\frac{dt}{d\ell} = t + \left(\frac{1}{T_c} - \frac{1}{\sqrt{2}T_c^2}\right)t^2 - \frac{4}{3T_c^4}t^3 + \frac{(8T_c - 7\sqrt{2})}{6T_c^6}t^4 + O(t^5)$ | $\frac{df}{d\ell} = 2f - 0.09664 - 0.7071x - 1.605x^2 - 0.8077x^3 + O(x^4)$ <br> $\frac{dx}{d\ell} = x + \frac{1}{2\sqrt{2}}x^2 - \left(\frac{3}{2} + \sqrt{2}\right)x^3 + \frac{1}{8}\left(4 + 3\sqrt{2}\right)x^4 + O(x^5)$ |
| $\frac{df}{d\ell} = 2f - 0.09664 - 3.414v - 43.25v^2 - 228.6v^3 + O(v^4)$ <br> $\frac{dv}{d\ell} = v - \left(34 + 24\sqrt{2}\right)v^3 - \frac{5}{6}\left(577 + 408\sqrt{2}\right)v^5 + O(v^7)$ | $\frac{df}{d\ell} = 2f - 0.09664 - 0.2071\tau - 0.1592\tau^2 + 0.01368\tau^3 + O(\tau^4)$ <br> $\frac{d\tau}{d\ell} = \tau + \frac{3\tau^3}{8} - \frac{7\tau^5}{48} + \frac{83\tau^7}{1024} + O(\tau^9)$ |

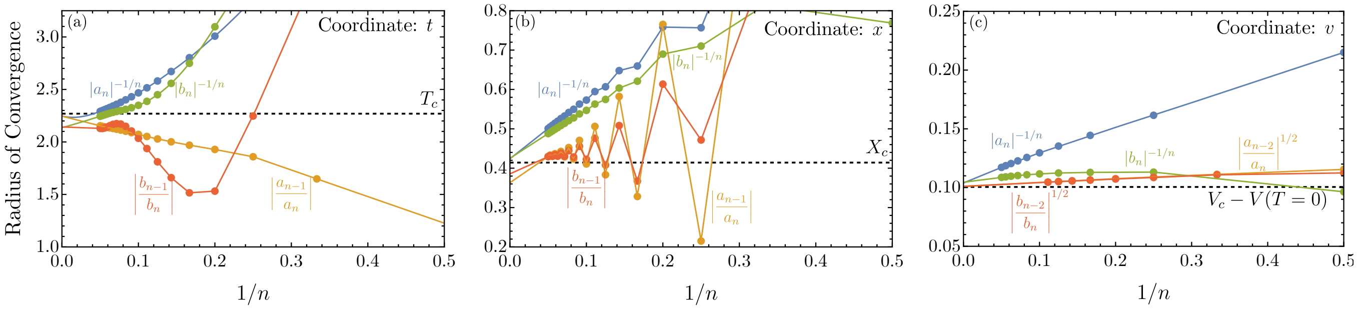


FIG. S1. Estimating the radii of convergence for expansions of Onsager's solution $a(t)\log t^2 + b(t)$ around the critical point. For expansion coordinates (a) $t$, (b) $x$, and (c) $v$, we compute the roots $|a_n|^{-1/n}$ (blue), $|b_n|^{-1/n}$ (green) and ratios $|a_{n-1}/a_n|$ (orange), $|b_{n-1}/b_n|$ (red) of the expansion coefficients. Note the Onsager solution is symmetric in the $v$-coordinate so in this case we use ratios $|a_{n-2}/a_n|$ and $|b_{n-2}/b_n|$. The solid lines show low-order interpolations (linear or quadratic depending on the apparent curvature of the points). In each case, the extrapolated radius of convergence is approximately equal to the distance from the critical point to zero-temperature. In coordinate $t$ and $x$ this distance is just $T_c$ and $X_c$ respectively, while in $v$ the distance is $V_c - V(T=0)$ because $V(T=0) = 8\sqrt{2} - 11 \neq 0$.

and $V = (5 - 3\sqrt{2} + X)/(1 + \sqrt{2} + X)$. The flows for the temperature coordinates can be obtained analytically, while the free energy flows (which include the analytic background) are evaluated numerically.

These RG flows correspond to the renormalization group transformation that has the 2D Ising critical point as its fixed point. In other words, all irrelevant parameters under this RG have zero amplitude at the 2D Ising critical point. For a different renormalization group the 2D Ising critical point lies on the stable manifold of its fixed point and there are irrelevant parameters that contribute corrections to scaling to the free energy. For the zero-field 2D Ising model, however, all these irrelevant parameters are *redundant*: they contribute corrections to scaling with integer exponents and are hence indistinguishable from analytic corrections. See Refs. [1–3] for an extended discussion of redundant parameters and Ref. [4] for an illustration (in the context of period-doubling iterated maps) of how modifying the renormalization group transformation can introduce redundant degrees of freedom.

### B. Estimating the radii of convergence for different expansion coordinates

In the main text, we claimed that the normal form expansions of Onsager's solution for the zero-field 2D Ising free energy have radii of convergence determined by the distance from the critical point to zero temperature. As a reminder, Onsager's solution can be expressed as $f(t) = a(t)\log t^2 + b(t)$ where $a$ and $b$ are analytic functions. We determinate these function perturbatively by expanding $f(t)$ around $T_c$ in different coordinates: $t = T - T_c$, $x = X - X_c$ and $v = V - V_c$, where $X = \exp(-2/T)$ and $V = (5 - 3\sqrt{2} + X)/(1 + \sqrt{2} + X)$. The critical points are respectively $T_c = -2/\log(1+\sqrt{2})$ and $X_c = V_c = -1 + \sqrt{2}$.

To estimate the radii of convergence for these expansions, we use the ratio and root tests for infinite series. Specifically, when the limits converge, the radius of convergence of a series $c(x) = \sum_{n=0}^{\infty} c_n x^n$ is given by $r = [\limsup_{n\to\infty} |c_n|^{1/n}]^{-1}$ (root test) or alternatively $r = \lim_{n\to\infty} |c_{n-1}/c_n|$ (ratio test). Examining these roots and ratios for a finite sequence of known coefficients therefore provides and estimate on the radius of convergence of the expansion of the functions $a$ and $b$. Fig. S1 shows the roots $|a_n|^{-1/n}$, $|b_n|^{-1/n}$ and ratios $|a_{n-1}/a_n|$, $|b_{n-1}/b_n|$ as a function of $1/n$ for expansions in $t$, $x$, and $v$. Extrapolating the $y$-intercept on these plots (i.e. the limit $n \to \infty$) gives an estimate of the radius of convergence.

While the expansions are not high enough order to determine the radius of convergence to high precision, in all cases the estimated radius is within a few percent of the distance from the critical point to zero temperature ($T_c$, $X_c$ and $V_c - V(T=0)$ respectively). Furthermore, the distance to zero temperature is well within the variation in estimated radii from different approaches and the expansion of $a$ versus $b$.

### C. Complex temperature phase portraits

In the main text we motivated the introduction of the coordinate, $V = (5 - 3\sqrt{2} + X)/(1 + \sqrt{2} + X)$, because this transformation extends the duality symmetry of the 2D Ising model to the complex temperature plane. In particular

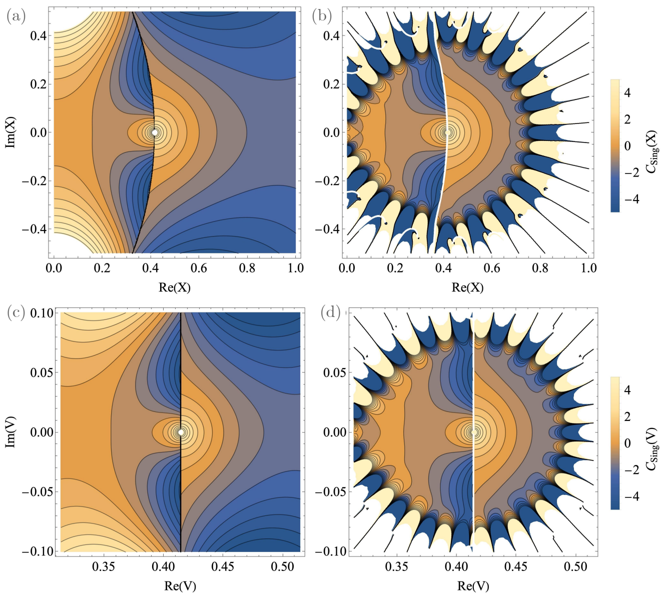


FIG. S2. Exact (a) & (c) and approximate (b) & (d) complex temperature specific heat $C_{\text{sing}} = \partial^2 F_{\text{sing}}/\partial\beta^2$ in coordinates $X = \exp(-2/T)$ (a)-(b) and $V = (5 - 3\sqrt{3} + X)/(1 + \sqrt{2} + x)$ (b)-(d). In the complex $X$-plane the singularities lie on a circle that passes through the critical point. The normal form expansion $\tilde{t}(x)$ attempts to bend the branch-cut of the logarithm to approximate this circle. In the complex $V$-plane the circle of singularities is mapped to a vertical line. The normal form expansion can capture this branch-cut at any order.

this linear fractional transformation straightens out the circle of Fisher zeros (zeros of the partition function) in the complex $X$-plane ($X = -1 + \sqrt{2}e^{i\theta}$, with $0 < \theta < 2\pi$) [5, 6], mapping them to a vertical line in the complex $V$-plane that intersects the critical point. Fig S2 shows contours of the singular part of the specific heat $C_{\text{sing}} = \partial^2 F_{\text{sing}}/\partial\beta^2$ in these complex $X$ and $V$ planes. We show both the exact solution and series approximation for each coordinate. The Fisher zeros become poles in the specific heat, so they are distinctly visible in these contours. As noted above, the coordinate transformation maps a circle of zeros in $X$ to a straight line in $V$. Interestingly, the series expansion in $x = X - X_c$ [Fig. S2(b)] approximates the circle of zeros before eventually breaking down. We conjecture that failure to fully capture these singularities contributes to the breakdown in convergence. Conversely, in $v = V - V_c$, the correct singularity is built into the expansion *and extended to the complex plane*, which allows convergence across all temperatures.

### D. Using low-order Onsager coefficients: Hybrid coefficient matching

In Fig. 2 of the main text, we mentioned that a hybrid matching schemes can be used to accelerate convergence if additional properties of the critical point are known. For example if low order coefficients in the Onsager solution are known, we can fix these and only use higher order terms in the expansion to match behavior at low and high temperatures. In other models, the (non-universal) amplitudes of the magnetization, specific heat, or susceptibility might be determined from high-precision Monte Carlo simulations and the low order coefficients in renormalization group flows (which are again non-universal) can in principle be computed via loop-expansions.

Fig. S3(a) shows that fixing the free-energy coefficients (analytic background and singular part) up to quadratic order to their exact values yields excellent convergence both at the critical point and at high/low temperatures with the maximal error in between (compare to Fig. 2(b) in the main text, where the error is maximum at the critical point). Leveraging additional information at the critical point improves the approximation by a factor of 3 to $10^3$ depending on order compared the case presented in the main text, where we only know the asymptotic scaling form at the critical point. In fact, the hybrid matching scheme accelerates convergence [Fig. S3(b)]: the exponential convergence rate (for the maximal error) is about 50% larger compared to only fitting to the low-temperature expansion.

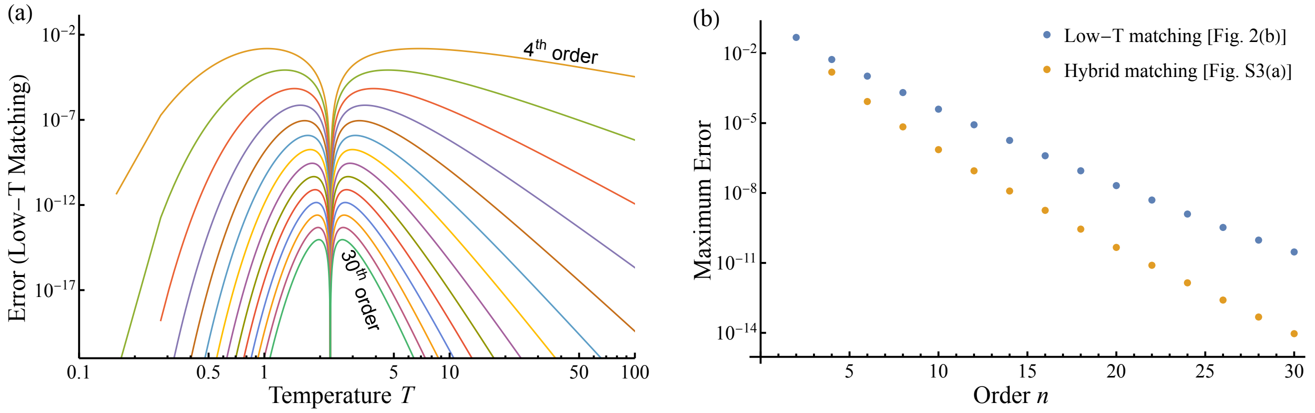


FIG. S3. Hybrid matching using knowledge about the critical point improves convergence. (a) The approximation error $|F_{\text{approx}} - F_{\text{sing}}|$ for the low-temperature matching expansion in coordinate $v$ (even orders $n = 4 - 30$) with coefficients up to quadratic order fixed to match Onsager's exact solution. At a given order the maximum error in this hybrid scheme is reduced compared to low-temperature matching with only the asymptotic scaling form [c.f. main text Fig. 2(b)]. (b) The maximum approximation error $\max_T |F_{\text{approx}} - F_{\text{sing}}|$ for the low-temperature and hybrid matching. Adding terms leads to exponential convergence to the exact free energy; the convergence rate is increased in the hybrid scheme.

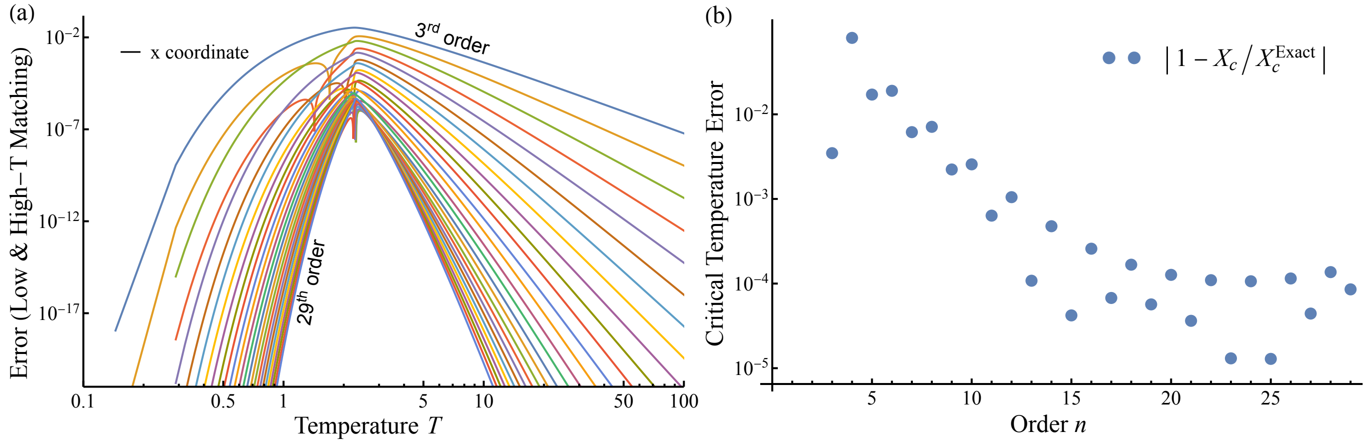


FIG. S4. Fitting 2D Ising free energy without knowledge of critical temperature $T_c$. (a) The approximation error $|F_{\text{approx}} - F_{\text{sing}}|$ for the low- and high-temperature matching expansion in coordinate $x = X - X_c$ (orders $n = 4 - 29$) with $X_c$ fit at each order as described in Section S1 E. These fits still obtain 7-digit accuracy, compared to 12-digits when $T_c$ is exactly known and the ideal dual-symmetric coordinate $v$ is used [c.f. main text Fig. 2(b)]. (b) The error in the estimated critical temperature $|1 - X_c/X_c^{\text{Exact}}|$ at each expansion order. Though convergence slows at high orders $X_c$ is still determined to within 0.01%.

### E. Fitting critical temperature

Here we demonstrate that fitting the critical temperature can be added to the coefficient matching procedure and still yield an exponentially convergent result. For this illustration we will work in the low temperature coordinate $x$ (using the dual-symmetric coordinate $v$ guarantees the correct critical temperature at all orders). As in the main text, we express the free energy as $f(x) = a(x) \log x^2 + b(x)$, with $x = X - X_c$ and expand analytic functions $a$ and $b$ order-by-order by matching to the expansion at zero and infinite temperature. For a given $X_c$ the matching is linear in coefficients $\{a_n\}$ and $\{b_n\}$ and can be solved exactly. We then perform a nonlinear least squares fit of the next zero temperature expansion coefficient by varying the critical temperature $X_c$. The resulting fitting error is shown in Fig. S4(a): even without knowledge of the critical temperature, we still obtain initial exponential convergence toward the exact solution, though the convergence slightly slows at high orders. The fit critical temperatures [Fig. S4(b)] also converges exponentially initially, achieving a $X_c$ estimate within 0.01% of the true value.

## S2. 3D ISING MODEL

### A. Background: Scaling theory and singular corrections

For completeness, here we provide a summary of how to incorporate normal form coordinate changes into systems with multiple relevant scaling variables (e.g. temperature and field) as well irrelevant variables. We will focus on the 3D Ising model and use the results to compute corrections to scaling for the zero-field free energy and magnetization. See Refs. [1, 7] for a broader review of this approach, including non-hyperbolic cases.

In contrast to the 2D Ising model, the renormalization group fixed point in three-dimensions is hyperbolic. There are no resonances or other bifurcations in 3D, so that all nonlinearities in the RG flow equations can be removed by normal form coordinate transformations. Including field $h$ and the leading irrelevant correction $u$, the flow equations (in terms of nonlinear scaling variables $\tilde{f}$, $\tilde{t}$, etc.) are

$$\frac{d\tilde{f}}{d\ell} = 3\tilde{f}, \qquad \frac{d\tilde{t}}{d\ell} = \lambda_t \tilde{t}, \qquad \frac{d\tilde{h}}{d\ell} = \lambda_h \tilde{h}, \qquad \frac{d\tilde{u}}{d\ell} = -\lambda_u \tilde{u}. \tag{S4}$$

There $\lambda_x > 0$, $x = t, h, u$ are the RG eigenvalues (or negative eigenvalue for $u$), which are related to standard critical exponents via $\lambda_t = 1/\nu$, $\lambda_h = \beta\delta/\nu$, and $\lambda_u = \omega$. These flow equations imply a variety of power-law invariant scaling combinations. The free energy has a power-law in $\tilde{t}$ times a universal scaling function of these invariant combinations [1]:

$$\tilde{f} = \tilde{t}^{2-\alpha}\mathcal{F}(\tilde{h}/\tilde{t}^{\beta\delta}, \tilde{u}\tilde{t}^{\theta}), \tag{S5}$$

where we have used the scaling relation $3\nu = 2-\alpha$ and introduce the irrelevant correction exponent $\theta = \nu\omega$. As in 2D, normal form theory tells us that the physical free energy can be obtained by writing the nonlinear scaling variables back in terms of physical temperature and field and adding the analytic background [7]. Here we treat the irrelevant parameter $u$ as a constant, absorbing any dependence of the nonlinear scaling variables on $u$ into the coefficients for temperature and field. To leading order the nonlinear scaling variables are linear in their physical counterparts: $\tilde{t}(t, h) = t(a + bt + ch^2 + \dots)$, with similar relations for $\tilde{h}$ and $\tilde{u}$. Note that $\tilde{t}$ is even in $h$: the temperature dependence of the system is invariant if we change the sign of the applied field. The leading irrelevant perturbation $\tilde{u}$ is also even in $h$. Inserting these transformations into Eq. (S5) we obtain,

$$f(t, h) = \tilde{t}(t, h)^{2-\alpha}\mathcal{F}(\tilde{h}(t, h)/\tilde{t}(t, h)^{\beta\delta}, \tilde{u}(t, h)\tilde{t}(t, h)^{\theta}) + f_a(t, h). \tag{S6}$$

Restricting this general scaling form to $h = 0$, we can extract the scaling for the zero-field free energy and magnetization $m = df/dh\big|_{h=0}$. Specifically, we find (suppressing the $h = 0$ arguments of scaling functions),

$$\begin{aligned} f(t) &= \tilde{t}(t)^{2-\alpha}\mathcal{F}_{\pm}(\tilde{u}(t)\tilde{t}(t)^{\theta}) + f_a(t) \\ m(t) &= \tilde{h}_1(t)\tilde{t}(t)^{\beta}\mathcal{M}(\tilde{u}(t)\tilde{t}(t)^{\theta}) \qquad t < 0. \end{aligned} \tag{S7}$$

Here, $\mathcal{F}_{\pm}(\tilde{u}\tilde{t}^{\theta}) = \lim_{h\to 0}\mathcal{F}(\tilde{h}/\tilde{t}^{\beta\delta}, \tilde{u}\tilde{t}^{\theta})$, which depends on the sign of $t$, $\mathcal{M}(Y) = d\mathcal{F}(X, Y)/dX\big|_{X=0}$, and $\tilde{h}_1(t) = d\tilde{h}/dh\big|_{h=0}$. Note that there is no analytic background in the magnetization because $m(t) \equiv 0$ for $t > 0$. Expanding these expressions to linear order in $\tilde{u}$ leads to the scaling forms given in the main text [Eq. (6)]:

$$\begin{aligned} f(t) &\approx A_{\pm}|\tilde{t}(t)|^{2-\alpha} + B_{\pm}\tilde{u}(t)|\tilde{t}(t)|^{2-\alpha+\theta} + f_a(t), \\ m(t) &\approx \tilde{h}_1(t)(|\tilde{t}(t)|^{\beta} + C\tilde{u}(t)|\tilde{t}(t)|^{\beta+\theta}) \qquad t < 0. \end{aligned} \tag{S8}$$

We take the critical exponents $\alpha$, $\theta$, and $\beta$ and universal amplitude ratios $A_+/A_-$ and $B_+/B_-$ as inputs for our theory. The functions $\tilde{t}(t)$, $\tilde{h}_1(t)$, $\tilde{u}(t)$, and $f_a(t)$ from normal form theory capture the analytic corrections to scaling (and analytic background) that can be fit to map out the entire phase.

### B. Low- and high-temperature fitting scheme

Following our work on the 2D Ising model, we fit the analytic corrections in Eq. (S8) by matching to low- and high-temperature expansions, working in coordinate $x = X - X_c$ with $X = \exp(-4/T)$. We find that fitting coefficients is more stable if we factor higher order terms in $\tilde{t}$ out of the power-laws. Specifically, since writing $\tilde{t} = t(1 + \delta\tilde{t}(t))$, we

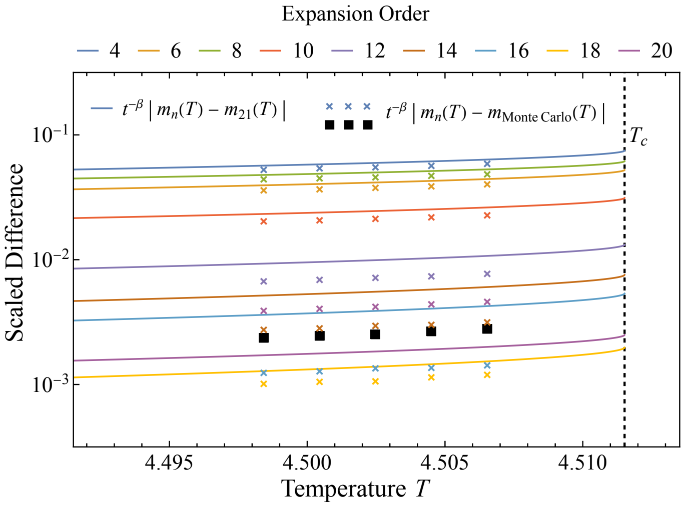


FIG. S5. Comparison of our magnetization approximations to the magnetization estimate from Monte Carlo simulations in Ref. [9]. We show the differences (scaled by the dominant power-law $t^{-\beta}$) between the $n^{\text{th}}$ order expansion and both (1) our best converged approximation $m_{21}(T)$ (solid lines) and (2) the Monte Carlo estimates (crosses). The black squares show the difference between the Monte-Carlo measurements and $m_{21}(T)$. As the approximations converge, they are also converging to the values measured in simulation; the distance to the data is within 30% of the estimated precision of our approximation (based on the difference between subsequent orders). Note the temperature range in this plot is very small and close to $T_c$, so the variation of fits and data after scaling by $t^{-\beta}$ is rather weak. This is also the regime where our convergence is slowest; it is furthest from the zero-temperature expansions used to fit the normal form transformation. Nonetheless we still obtain an approximation with absolute errors less than $2 \cdot 10^{-3} \times t^{\beta}$.

have $|\tilde{t}(t)|^p = A(t)|t|^p$, where $A(t) = (1 + \delta\tilde{t}(t))^p$ is analytic. Furthermore, for the 3D Ising model, it is known that there is a complex pole in the free energy that lies closer to zero temperature than to the critical point. This pole leads to the well-known divergence in the low-temperature expansion and naturally shows up in traditional dLog-Padé approximates [8]. We factor this pole out of the analytic expansions in Eq. (S8), and fit its location, which dramatically improves the stability the fit coefficients. Finally, rather than matching low- and high-temperature expansions exactly, we use Levenberg–Marquardt least squares fitting to determine the normal form coordinate transformations; again this approach offers greater stability, especially with the nonlinearities introduced by the pole mentioned above.

As noted in the previous section, we take the universal critical exponents and amplitude ratios as inputs to our approach. To our knowledge, the ratio $B_+/B_-$ is not well constrained in the literature; therefore we neglect the correction to scaling for the free energy fit. In the magnetization, we assume a constant coefficient for the correction to scaling. With these assumptions, we use the following simplified version of Eq. (S8) for the free energy and magnetization,

$$
\begin{aligned}
f(x) &= \frac{F(x)}{x - x_p} A_\pm |x|^{2-\alpha} + \frac{f_a(x)}{x - x_p} \\
m(x) &= \frac{M(x)}{x - x_p} |x|^{\beta} + \frac{u_0}{x - x_p} |x|^{\beta+\theta} \qquad x < 0.
\end{aligned}
\tag{S9}
$$

We expand $F$, $f_a$ and $M$ as power series and fit these coefficients, the pole $x_p$ and singular correction amplitude $u_0$ by matching to low- and high-temperature coefficients. As shown in Fig. 3 in the main text, the fits are self-consistent: they converge the difference between subsequent approximations converge exponentially. For the free energy our approximation converges to within the precision allowed by the uncertainty in the amplitude ratio $A_+/A_- \approx 0.536 \pm 0.002$: the difference in approximation due to this uncertainty is comparable to the difference in approximations of increasing order. For the magnetization our result compares favorably with dLog-Padé approximation near zero-temperature [8] and with fits to Monte Carlo simulations of the form $m(x) = |x|^{\beta}(a + b|x| + c|x|^{\theta})$, which include the leading singular correction [10]. As mentioned in the main text, this later estimate is more accurate near the critical point because it includes the leading singular correction. We also compared to the high-precision Monte Carlo estimates of the magnetization near the critical point from Ref. [9] (red cross in Fig. 3). Fig. S5 shows an expanded comparison between this data and our fit magnetization. Here we see that as our approximation order increases and approaches the best approximation $m_{21}(T)$ the solutions are also approaching the numerically measured magnetization. The distance to these Monte Carlo estimates is comparable to the estimated precision of the approximation. High-precision Monte

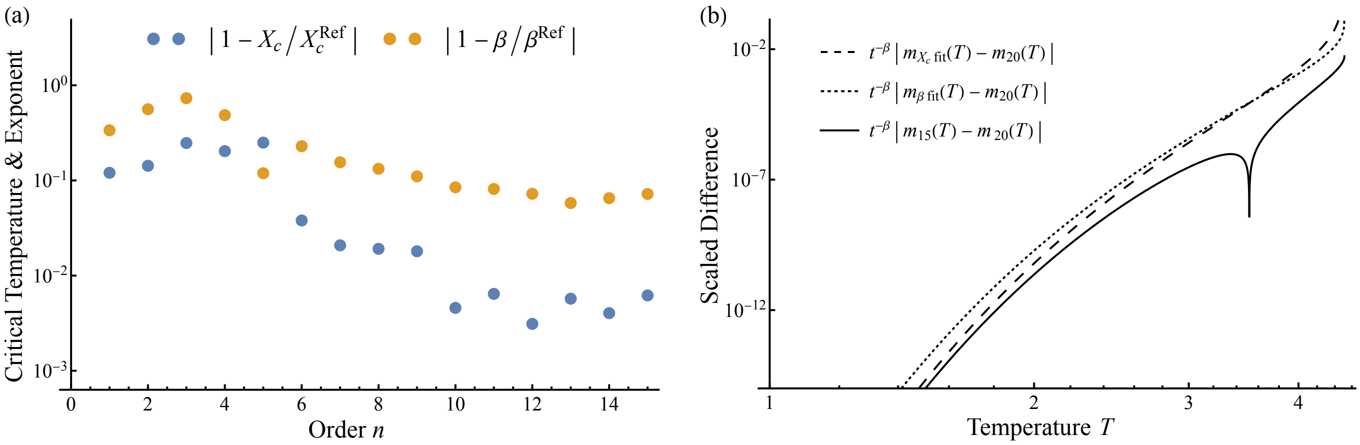


FIG. S6. Fitting 3D Ising magnetization without knowledge of critical temperature $T_c$ or critical exponent $\beta$. (a) The fit critical temperature and exponents compared to literature values $X_c^{\text{Ref}} = 0.41205$ [10] and $\beta^{\text{Ref}} = 0.326419$ [11] Critical temperature and exponent are determined within 0.5% and 10% respectively. (b) The corresponding magnetization curves (order $n = 15$) for $X_c$ fitting (dashed), $\beta$ fitting (dotted) compared best converged magnetization fit $m_{20}(T)$ with $X_c$ and $\beta$ known. For reference we show the corresponding fit error when critical temperature and exponent are known (solid). Far from the critical point the magnetization estimate remains highly accurate, though one loses roughly a factor of 10 in accuracy if one does not have an independent measure of the critical temperature (similarly for the critical exponent).

Carlo estimates like these could also be incorporated into the normal form fitting procedure, similar to the hybrid fits shown in Section S1 D. To this end, the least squares fitting described here can easily incorporate additional data of this type and account for statistical errors in such measurements.

### C. Fitting critical temperature and exponents

As in the 2D Ising model, we investigate the performance of the normal form expansion of the 3D Ising scaling when the critical temperature or exponents are not known. As an example, we will focus on the magnetization, fitting the expansion in $x = X - X_c$ given in Eq. (S9), but including critical temperature $X_c$ or leading critical exponent $\beta$ as parameters in the least squares fitting. For this illustration we neglect the singular correction to scaling (i.e. fix $u_0 = 0$).

Fig. S6(a) shows the fit critical temperature (assuming exponents are known) or critical exponent (assuming $X_c$ is known) compared to high-precision estimates from the literature [10, 11]. Fitting gives the correct critical temperature within 0.5% and critical exponent within 10%. The Padé estimate of the exponent $\beta$ at the corresponding order is about twice as accurate [8]. Fig. S6(b) shows the corresponding magnetization predictions at order $n = 15$ compared to the best converged fit when $X_c$ and $\beta$ are assumed to be known (dashed, dotted lines). These fits are comparable to the convergence of the $15^{\text{th}}$-order approximation when critical temperature and exponents are given (solid line). The largest deviation comes near $T_c$ where the magnetization estimate (scaled by the dominant power-law $t^{-\beta}$) is worse by a few orders of magnitude. Far from the critical point, ignorance of either the critical temperature or critical exponent only reduces accuracy by about one order of magnitude.

While the critical temperature and exponent fits are not competitive with refined techniques for the 3D Ising model, we conjecture that improvements to our approach might also yield more precise estimates of the critical temperature and exponents. Directions for future study include: (1) varying the relative orders between leading singularity and correction to scaling expansions, (2) incorporating additional complex-temperature poles, (3) exploring different nonlinear fitting schemes, and (4) looking for more suitable expansion coordinates (which we have shown is useful in 2D).


[1] J. P. Sethna, D. Hathcock, J. Kent-Dobias, and A. Raju, Normal forms, universal scaling functions, and extending the validity of the RG, arXiv preprint arXiv:2304.00105 (2023).
[2] R. H. Swendsen, Optimization of real-space renormalization-group transformations, Phys. Rev. Lett. **52**, 2321 (1984).
[3] M. E. Fisher and M. Randeria, Location of renormalization-group fixed points, Phys. Rev. Lett. **56**, 2332 (1986).

[4] A. Raju and J. P. Sethna, Reexamining the renormalization group: Period doubling onset of chaos, arXiv preprint arXiv:1807.09517 (2018).

[5] M. E. Fisher, The nature of critical points, in *Boulder Lectures in Theoretical Physics: Statistical Physics, Weak Interactions, Field Theory*, Vol. 7c (University of Colorado Press, 1964) pp. 1–159.

[6] B. P. Dolan, W. Janke, D. A. Johnston, and M. Stathakopoulos, Thin Fisher zeros, Journal of Physics A: Mathematical and General **34**, 6211 (2001).

[7] A. Raju, C. B. Clement, L. X. Hayden, J. P. Kent-Dobias, D. B. Liarte, D. Z. Rocklin, and J. P. Sethna, Normal form for renormalization groups, Phys. Rev. X **9**, 021014 (2019).

[8] J. W. Essam and M. E. Fisher, Padé Approximant Studies of the Lattice Gas and Ising Ferromagnet below the Critical Point, The Journal of Chemical Physics **38**, 802 (1963).

[9] M. Hasenbusch, Thermodynamic casimir effect: Universality and corrections to scaling, Phys. Rev. B **85**, 174421 (2012).

[10] A. L. Talapov and H. W. J. Blöte, The magnetization of the 3d ising model, Journal of Physics A: Mathematical and General **29**, 5727 (1996).

[11] F. Kos, D. Poland, D. Simmons-Duffin, and A. Vichi, Precision islands in the Ising and O(N) models, Journal of High Energy Physics **2016**, 36 (2016).
